# Supplementary material for: Large Out-of-Plane Piezoelectric Effect in Janus Ferromagnetic Semiconductor Monolayer of CrOFBr
Source: arXiv:2406.06265 source file (2024-06-10)
Supplement: Supplementary file 1 [file supplementary_material.pdf]

# Supporting Information

## Large Out-of-Plane Piezoelectric Effect in Janus Ferromagnetic Semiconductor Monolayer of CrOFBr

*Qiuyue Ma, Guochun Yang, Busheng Wang , and Yong Liu**

*State Key Laboratory of Metastable Materials Science and Technology & Key Laboratory for Microstructural Material Physics of Hebei Province, School of Science, Yanshan University, Qinhuangdao, 066004, P.R. China*

+ corresponding author:
Electronic mail: yongliu@ysu.edu.cn

(a) CrOClBr (b) CrOFCl

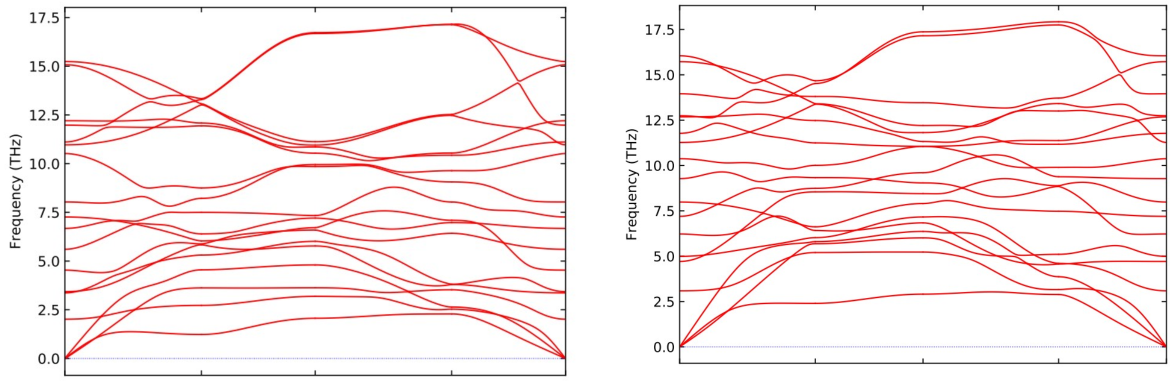


Figure S1. Phonon spectrum of Janus (a) CrOClBr and (b) CrOFCl monolayers.

(a) CrOClBr (b) CrOFCl

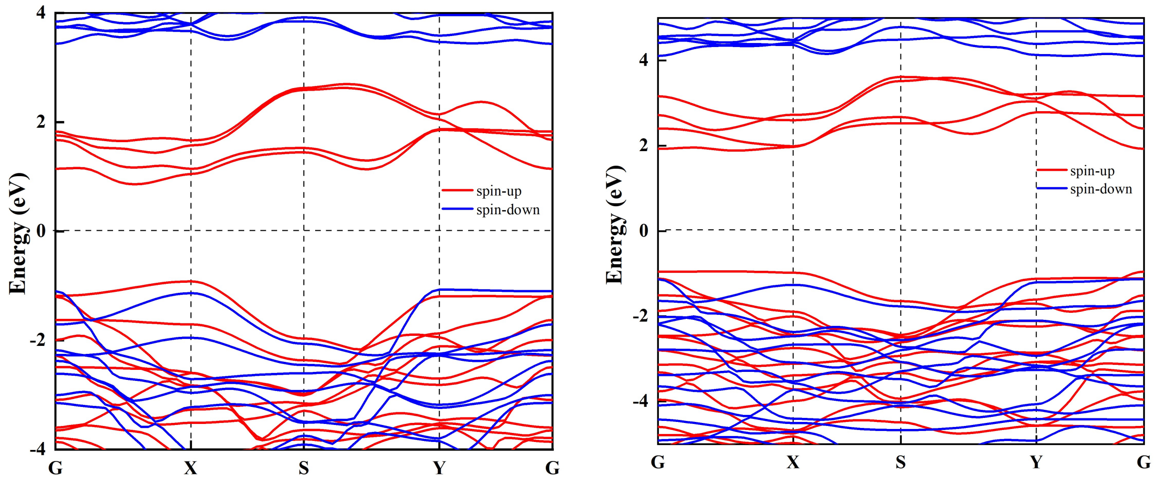


Figure S2. Energy band structures of Janus (a) CrOClBr and (b) CrOFCl monolayers.

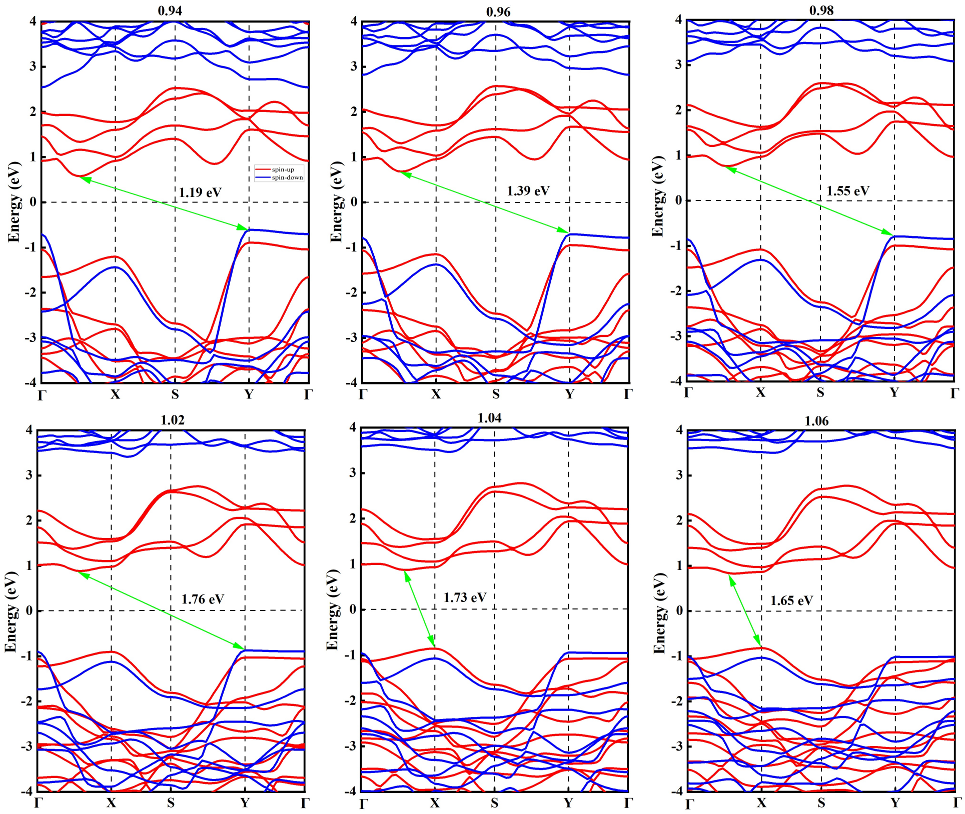


Figure S3. Energy band structures of Janus CrOFBr monolayer with $a = a_0$ changing from 0.94 to 1.06.

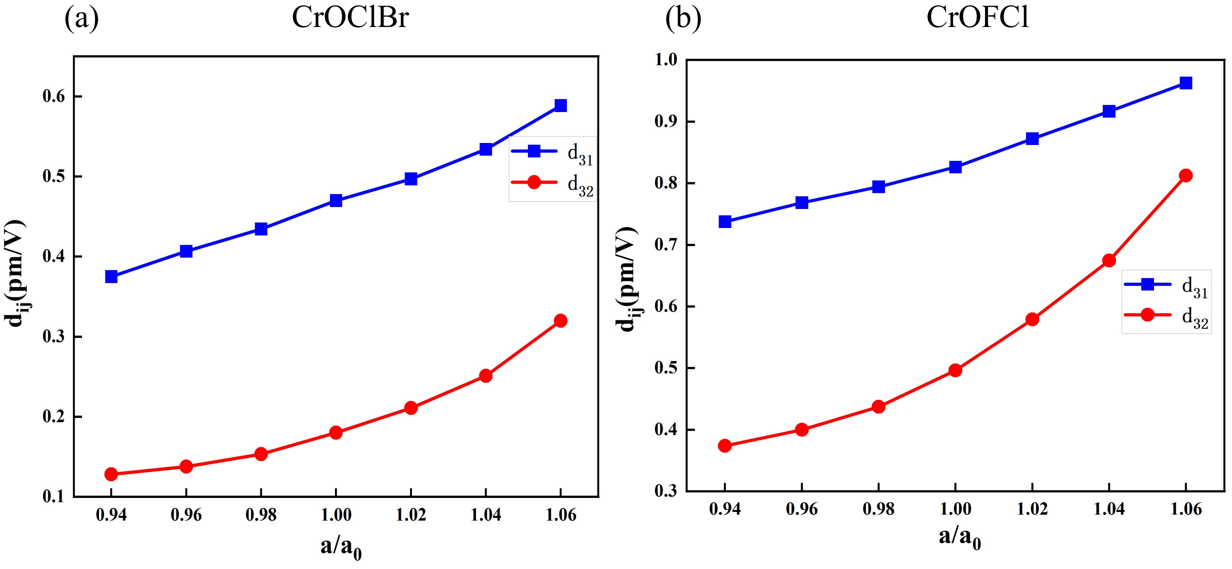


Figure S4. Piezoelectric strain coefficients of Janus CrOClBr and CrOFCl monolayers as a function of $a = a_0$ changing from 0.94 to 1.06.
